# Supplementary material for: Interpretable Sentence Representation with Variational Autoencoders and Attention
Source: arXiv:2305.02810 source file (2023-05-04)
Supplement: Supplementary file 1 [file appendix01.tex]

\noindent The following scripts are the code that I used for the training of \textit{traditional word embedding models} (i.e., PPMI-SVD, SGNS) and \textit{similarity-based estimation}.

\begin{lstlisting}[style=py, caption=Python code for the word embedding by using the PPMI-SVD model]

class PPMI_SVD_Algorithm:

    def __init__ (self, fold, postposition, postposition_ko, window):
        self.fold = fold
        self.postposition = postposition
        self.postposition_ko = postposition_ko
        self.window = window


\end{lstlisting}
